# Supplementary material for: Who Wrote this Code? Watermarking for Code Generation
Source: arXiv:2305.15060 source file (2024-07-03)
Supplement: Supplementary file 1 [file alg_thres_select.tex]

\begin{algorithm}[ht!]
\caption{Determine Entropy Threshold for \myalgo}\label{alg:thres_select}
\begin{algorithmic}[1]
\STATE{\bfseries Input:} Batch of text data $D$,

Watermark parameters $\gamma, \delta$,

Target green token ratio value of watermarked text $\phi$
\STATE{\bfseries Output:} Entropy threshold $\threshold$

\STATE Apply LLM for each text in $D$ to get a set of probability distribution vectors $\{ p_1,\dots p_n\}$.

\STATE Compute entropy values $\boldsymbol{H}=\{H_1,\dots,H_n\}$ from each probability vector $p$.

\STATE Compute $\boldsymbol{P_G}$ based on each token, which is how likely a token sampled from the watermarked version of each probability vector $p$ will be a green token; Approximate by repetitive calculation using random green list.

\begin{align}
\Sigma_{k \in G}\mathbb{E}_{G,R} \frac{e^\delta p_k}{\Sigma_{i \in R}p_i + e^\delta \Sigma_{i \in G}p_i}\nonumber
\end{align}

\STATE Regard the data of entropy($\boldsymbol{H}$) and empirical set of probability of green tokens($\boldsymbol{P_G}$) as unnormalized joint discrete distribution $P(\boldsymbol{H},\boldsymbol{P_G})$, The entropy threshold $\threshold$ is the solution of the equation below:
\begin{align}
\phi = \frac{\Sigma \boldsymbol{P_G} P(\boldsymbol{H},\boldsymbol{P_G}|\boldsymbol{H}\ge\threshold)}{\Sigma P(\boldsymbol{H},\boldsymbol{P_G}|\boldsymbol{H}\ge\threshold)}\nonumber
\end{align}
\end{algorithmic}
\end{algorithm}
