# Supplementary material for: Who Wrote this Code? Watermarking for Code Generation
Source: arXiv:2305.15060 source file (2024-07-03)
Supplement: Supplementary file 2 [file tab_entropy_calibration.tex]

\begin{table}[t]
\centering
\begin{tabular}{|c|c|c|c|c|}
\hline
\textbf{\parbox{1.5cm}{\centering entropy \\ threshold}} & $E[N^h/N]$ & $E[N^h_G/N^h]$ & $z'$ \\ \hline
0.032 & 0.706 & 0.5 & 0.485 \\ \hline
0.279 & 0.497 & 0.6 & 0.570 \\ \hline
0.734 & 0.337 & 0.7 & 0.603 \\ \hline
0.820 & 0.311 & 0.72 & 0.606 \\ \hline
0.871 & 0.299 & 0.73 & 0.606 \\ \hline
0.980 & 0.275 & 0.75 & 0.605 \\ \hline
1.094 & 0.252 & 0.77 & 0.603 \\ \hline
1.156 & 0.241 & 0.78 & 0.601 \\ \hline
1.227 & 0.229 & 0.79 & 0.597 \\ \hline
\end{tabular}
\caption{The relation between the entropy threshold and $z’=E[\frac{N^h}{N}] (E[\frac{N^h_G}{N^h}]-\gamma)$. We set $\gamma$=0.25 and $\delta$=3.0.}
\label{tab:entropy_calibration}
\end{table}
